# Supplementary material for: Learning Counterfactual Representations for Estimating Individual Dose-Response Curves
Source: arXiv:1902.00981 source file (2020-12-10)
Supplement: Supplementary file 1 [file appendix.pdf]

# Supplementary Material for: Learning Counterfactual Representations for Estimating Individual Dose-Response Curves

**Patrick Schwab**[1], **Lorenz Linhardt**[2], **Stefan Bauer**[3], **Joachim M. Buhmann**[2], **Walter Karlen**[1]
[1]Institute of Robotics and Intelligent Systems, ETH Zurich, Switzerland
[2] Department of Computer Science, ETH Zurich, Switzerland
[3] MPI for Intelligent Systems, Tübingen, Germany
patrick.schwab@hest.ethz.ch

## A Treatment Assignment Bias Regularisation

To address treatment assignment bias in DRNets, we evaluated four different regularisation strategies: (1) distribution matching between treatment groups using the Wasserstein regulariser (+ Wasserstein), (2) propensity dropout (+ PD), (3) matching on the entire dataset, and (4) matching on the batch level. Because neither of these regularisation strategies were originally developed for the setting with parametric treatment options, we implemented näive extensions thereof for this setting. To extend (1) to this setting, we followed Schwab et al. (2018) and penalised pair-wise differences between treatment group distributions in the topmost shared hidden layer using the first treatment option as the control treatment. For (2), we applied PD for each treatment option to both the corresponding per-treatment layers and to the respective treatment option's head layers in each dosage stratum. To use (3) dataset-wide and (4) per-batch matching with parametric treatments, we followed the PM algorithm outlined in Schwab et al. (2018), and matched directly on the covariates $X$ with the dosage parameter $s$ added to the covariate set. For datasets of dimensionality higher than 200, we matched on a low-dimensional representation obtained via Principal Components Analysis (PCA) using 50 principal components in order to reduce the computational requirements.

## B Hyperparameters

We used a standardised approach to hyperparameter optimisation for all methods. Each method was given exactly the same amount of hyperparameter optimisation runs (5 on TCGA, and 10 on all other benchmarks). We also fixed the random seed such that all methods were evaluated on exactly the same random hyperparameter configurations. For the methods based on neural network models (DRNet, + Repeat, + Wasserstein, + PD, + PM, + $\text{PSM}_{\text{PM}}$, MLP, TARNET, GANITE), we chose hyperparameters at random from predefined ranges (Table S1). For "+ Wasserstein", we additionally chose an imbalance penalty weight at random from 0.1, 1.0, or 10.0. For GANITE, we also randomly chose the supervised loss weights $\alpha$ and $\beta$ from 0.1, 1.0, and 10.0 (Yoon et al., 2018) as an additional hyperparameter. For BART and CF, we used the default hyperparameters from their respective implementations in the R-packages "bartMachine" (Kapelner & Bleich, 2013) and "grf" (Athey et al., 2016). Because CF was designed for estimating the difference in treatment effect between two treatment options and not for directly estimating treatment outcomes $\hat{y}_t$, we used a baseline ridge regression model with regularisation strength $\alpha = 0.5$ to estimate a control outcome $\hat{y}_0$ for the first treatment and one CF model to estimate the difference in treatment effect between that control treatment and all other treatment options (Schwab et al., 2018). For KNN, we used 5 nearest neighbours to compute the potential outcomes matching on the covariates $X$ with the dosage parameter $s$ added as an additional covariate. For GPS, we used the implementation in the "causaldrf" R-package (Galagate, 2016) with a normal treatment model, a linear treatment formula,

Table S1: Hyperparameter ranges used in our experiments.

| Hyperparameter | Values |
|---|---|
| Batch size $B$ | 32, 64, 128 |
| Number of units per hidden layer $M$ | 24, 48, 96 |
| Number of hidden layers $L$ | 2, 3 |
| Dropout percentage $p_{\text{dropout}}$ | $[0.0, 0.2]$ |

and a polynomial of degree 2 as the outcome formula. To reduce the computational requirements for GPS to a manageable level, we additionally preprocessed the covariates $X$ using PCA dimensionality reduction with 16 principal components for benchmarks with a covariate-space dimensionality higher than 200.

## C Computing Infrastructure

We used computing infrastructure consisting of compute nodes with Intel i5 and Xeon CPUs to run the experiments described in this paper.

## D Dosage Policy Error and Policy Error Results

We report the Dosage Policy Error (DPE) and Policy Error (PE) results in Tables S2 and S3, respectively. We found that DRNets outperformed all existing state-of-the-art methods in terms of DPE and PE with the exception of the PE on News-8, where DRNets achieved the second-best result after GPS.

Table S2: Comparison of methods for counterfactual inference with multiple parametric treatments on News-2/4/8/16, MVICU and TCGA. We report the mean value ± the standard deviation of $\sqrt{\text{DPE}}$ on the respective test sets over 5 repeat runs with new random seeds. n.r. = not reported for computational reasons (excessive runtime). $^{\dagger}$= significantly different from DRNet ($\alpha < 0.05$).

| Method | News-2 | News-4 | News-8 | News-16 | MVICU | TCGA |
|---|---|---|---|---|---|---|
| DRNet | 14.0 ± 0.1 | 14.3 ± 0.2 | 17.2 ± 0.6 | 19.1 ± 2.1 | **5.0** ± 1.5 | 2.1 ± 0.4 |
| - Repeat | 17.5 ± 7.1 | †18.5 ± 3.8 | 16.8 ± 2.9 | **16.1** ± 3.0 | 5.4 ± 3.1 | 5.4 ± 3.9 |
| + Wasserstein | †13.8 ± 0.1 | 14.2 ± 0.3 | **16.7** ± 0.6 | 18.7 ± 2.4 | 20.3 ± 19.0 | 2.9 ± 1.3 |
| + PD | †**13.7** ± 0.1 | 14.3 ± 0.2 | 17.6 ± 0.0 | 16.5 ± 2.0 | †38.9 ± 19.6 | †12.7 ± 5.4 |
| + PM | †**13.7** ± 0.1 | **13.9** ± 0.5 | †21.3 ± 2.7 | 21.0 ± 0.7 | †12.5 ± 3.5 | **1.8** ± 0.1 |
| + $\text{PSM}_{\text{PM}}$ | 14.0 ± 0.1 | 14.3 ± 0.1 | †19.5 ± 1.3 | 19.2 ± 1.6 | †28.1 ± 1.4 | 2.5 ± 1.1 |
| MLP | †47.1 ± 0.0 | †43.2 ± 0.1 | †39.8 ± 0.4 | †40.7 ± 0.0 | †42.8 ± 22.8 | †31.1 ± 0.1 |
| TARNET | †45.0 ± 1.1 | †41.5 ± 1.1 | †38.6 ± 1.1 | †38.1 ± 1.4 | †106. ± 48.8 | †38.6 ± 1.1 |
| GANITE | †39.4 ± 0.1 | †35.5 ± 0.1 | †32.6 ± 0.2 | †32.0 ± 0.3 | †103. ± 9.1 | †26.5 ± 0.6 |
| kNN | †44.6 ± 0.0 | †41.4 ± 0.0 | †39.2 ± 0.0 | †38.1 ± 0.0 | †60.5 ± 0.0 | n.r. |
| GPS | †42.3 ± 0.0 | †34.7 ± 0.0 | †22.5 ± 0.0 | 17.3 ± 0.1 | †81.6 ± 0.0 | †23.8 ± 0.0 |
| CF | †47.1 ± 0.0 | †43.2 ± 0.0 | †38.3 ± 0.0 | †35.2 ± 0.0 | †116. ± 0.0 | †30.9 ± 0.0 |
| BART | †31.6 ± 1.4 | †25.0 ± 1.5 | †23.1 ± 0.4 | n.r. | †39.9 ± 2.4 | n.r. |

Table S3: Comparison of methods for counterfactual inference with multiple parametric treatments on News-2/4/8/16, MVICU and TCGA. We report the mean value ± the standard deviation of $\sqrt{\text{PE}}$ on the respective test sets over 5 repeat runs with new random seeds. n.r. = not reported for computational reasons (excessive runtime). $^{\dagger}$= significantly different from DRNet ($\alpha < 0.05$).

| Method | News-2 | News-4 | News-8 | News-16 | MVICU | TCGA |
|---|---|---|---|---|---|---|
| DRNet | 15.7 ± 0.2 | 15.5 ± 0.4 | 15.1 ± 0.2 | 19.2 ± 14.9 | 12.9 ± 1.2 | **2.1** ± 0.1 |
| - Repeat | 20.4 ± 9.6 | 20.0 ± 10. | 24.3 ± 12. | 5.3 ± 8.8 | 13.7 ± 2.5 | 2.9 ± 1.3 |
| + Wasserstein | †15.2 ± 0.1 | 15.4 ± 0.5 | 15.6 ± 1.1 | 19.2 ± 14.9 | 13.6 ± 1.3 | 2.2 ± 0.0 |
| + PD | 15.3 ± 0.6 | †32.8 ± 0.0 | 14.9 ± 0.0 | † **0.9** ± 0.0 | †48.1 ± 27.1 | †21.8 ± 9.2 |
| + PM | †**15.1** ± 0.1 | **12.4** ± 5.3 | †29.3 ± 7.2 | 33.0 ± 11.7 | **12.1** ± 1.9 | 2.3 ± 0.4 |
| + $\text{PSM}_{\text{PM}}$ | †16.2 ± 0.4 | 15.3 ± 0.3 | †23.7 ± 7.3 | † 1.3 ± 0.8 | †23.3 ± 4.7 | †2.3 ± 0.1 |
| MLP | †49.5 ± 0.1 | †49.6 ± 0.0 | †48.5 ± 0.7 | †48.3 ± 0.3 | †23.7 ± 9.8 | †37.1 ± 2.3 |
| TARNET | †47.2 ± 2.1 | †48.0 ± 1.8 | †47.7 ± 1.1 | †44.8 ± 3.2 | †102. ± 44.0 | †47.7 ± 1.1 |
| GANITE | †42.6 ± 0.3 | †40.3 ± 0.3 | †42.7 ± 0.4 | 34.4 ± 0.6 | †96.7 ± 9.9 | †25.9 ± 1.1 |
| kNN | †45.2 ± 0.0 | †42.1 ± 0.0 | †45.5 ± 0.0 | †46.4 ± 0.0 | †59.1 ± 0.0 | n.r. |
| GPS | †44.6 ± 0.0 | †13.3 ± 0.0 | †**13.3** ± 0.0 | †1.6 ± 0.0 | †140. ± 0.0 | †20.0 ± 0.0 |
| CF | †48.9 ± 0.0 | †49.6 ± 0.0 | †49.6 ± 0.0 | †48.3 ± 0.0 | †108. ± 0.0 | †35.3 ± 0.0 |
| BART | †35.5 ± 14. | †34.6 ± 4.2 | †44.5 ± 1.2 | n.r. | 13.2 ± 1.0 | n.r. |
